# Supplementary material for: MC-GTA: Metric-Constrained Model-Based Clustering using Goodness-of-fit Tests with Autocorrelations
Source: arXiv:2405.18395 source file (2024-06-03)
Supplement: Supplementary file 1 [file 6-ablation_study.tex]

% \vspace{-0.3cm}
\subsection{Comparing Feature Distance Metrics}
\label{sec:ablation-visualization}
Here we present a simple experiment to show how a model-based approach outperforms simple Euclidean distance/cosine distance when the underlying model is properly selected. Figure~\ref{fig:ablation-feature-distance} depict the histograms of pairwise Wasserstein-2 distance, Euclidean distance, and cosine distance between two observations in the Pavement dataset, which is a time series that well satisfies the conditions of the model-based approach. 
The blue represents intra-cluster pairs and the orange represents inter-cluster pairs. We can see the model-based Wasserstein-2 distance itself makes distinguishing intra-cluster and inter-cluster pairs a lot easier than using Euclidean or cosine distance.  It clearly demonstrates that the raw distance by itself can be very unreliable when there are complex patterns in the metric space (e.g. those in motion sensor signals).

Besides the disadvantages compared with the model-based approach listed above, Euclidean and cosine distances have their intrinsic drawbacks, too. Euclidean distance is known to be inefficient in high dimensions due to sparsity (see~\citep{aggarwal2001surprising} for a review). The cosine distance is the worst-performing metric here because it only considers angles between observations, while the Pavement dataset accounts for magnitude as well.

\begin{figure*}[ht!]
\centering
\vspace{-0.2cm}
\subfloat[\rebut{Cosine distance}]{\includegraphics[width = 0.3\textwidth]{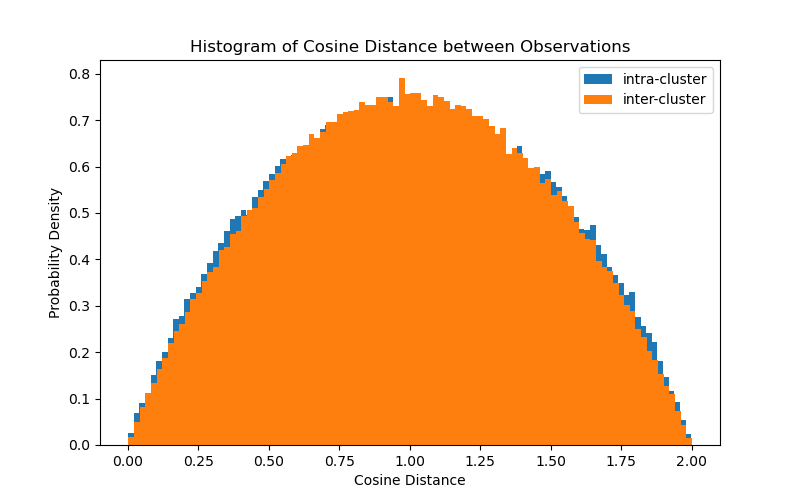}\label{fig:cosine-hist}}
\subfloat[\rebut{Euclidean distance}]{\includegraphics[width = 0.3\textwidth]{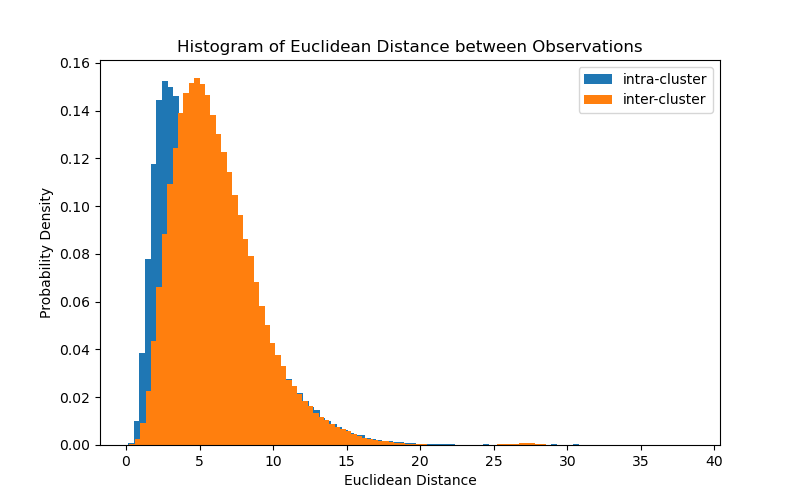}\label{fig:euclidean-hist}}
\subfloat[\rebut{Wasserstein-2 distance}]{\includegraphics[width = 0.3\textwidth]{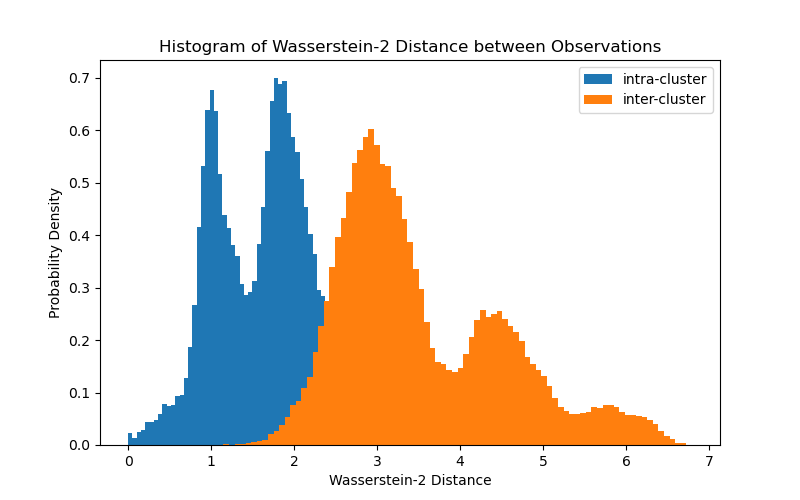}\label{fig:wasserstein-hist}}
\vspace{-0.2cm}
\caption{\rebut{The histogram of pairwise distances between intra-cluster and inter-cluster observations  for the Pavement dataset.
Here model-based Wasserstein-2 distance outperforms cosine distance and Euclidean distance in distinguishing inter-cluster and intra-cluster observations. 
The histograms (i.e., the empirical distribution) of intra/inter-cluster Wasserstein-2 distance have very different patterns (different means, variances and modes), thus it is more informative to use Wasserstein-2 distance in distance-based clustering.
}}
\label{fig:ablation-feature-distance}
\end{figure*}
